# Supplementary material for: UEyes: An Eye-Tracking Dataset across User Interface Types
Source: arXiv:2402.05202 source file (2024-02-07)
Supplement: Supplementary file 1 [file REMOVE10-Appendix.tex]

\section{Overall Location and Color Bias}

\subsection{Effect of Location}
\label{sec:analysis-location}

\autoref{fig:location_bias} shows the spatial distribution of eye fixations across the quadrants of the screen viewport.
We did not observe a center location bias, since fixations were particularly skewed towards top-left part of the screen,
This finding is similar to previous work that analyzed visual saliency on webpages~\cite{shen2014webpage} and mobile UIs~\cite{leiva2020understanding}.

\begin{figure*}[!ht]
  \def\w{0.32\linewidth}
  \centering

  \subfloat[Up to 1 second]{\includegraphics[width=\w]{results/dataset-first1s.csv_location_bias}}\hfill
  \subfloat[Up to 3 seconds]{\includegraphics[width=\w]{results/dataset-first3s.csv_location_bias}}\hfill
  \subfloat[Up to 7 seconds]{\includegraphics[width=\w]{results/dataset.csv_location_bias.pdf}}
  \caption{
    Location bias analysis.
    The thick dashed lines denote the middle of the screen viewport along the X and Y axis.
  }
  \Description{Color brightness analysis.}
  \label{fig:location_bias}
\end{figure*}

\begin{figure}[!ht]
  \def\w{0.24\linewidth}
  \centering

  \subfloat{\includegraphics[width=\w]{results/quadrants-first1s.csv_boxplot.pdf}}
  \subfloat{\includegraphics[width=\w]{results/quadrants-first3s.csv_boxplot.pdf}}
  \subfloat{\includegraphics[width=\w]{results/quadrants.csv_boxplot.pdf}}

  \caption{
    Location bias analysis.
    Distribution of fixations in screen quadrants.
    Q1: top-right, Q2: top-left, Q3: bottom-left, Q4: bottom-right.
  }
  \Description{Quadrant fixations analysis.}
  \label{fig:quadrants}
\end{figure}

We show saliency location bias analysis up to 7s for images from different categories (posters, mobile UIs, desktop UIs, webpages) in~\autoref{fig:location_bias_diff_categories}. The two top quadrants attracted more fixations than the bottom quadrants for all the categories. Desktop UIs and webpages particularly attract people to focus on the bottom part and pay much less attention to the bottom part, while people prefer to view mobile UIs from top to bottom leading to a vertical location bias.  

The top-left quadrant (Q2) attracted significantly more fixations than any other part of the display,
followed by the top-right (Q1), bottom-left (Q3), and bottom-right (Q4) quadrants.
The omnibus test revealed a statistically significant difference
between the average number of fixations per user and visual content for each of the quadrants
except for the `First fixation' scenario; see \autoref{tbl:quadrants}.
Effect sizes $\phi$ suggest a high practical importance of the differences~\cite{kim2017effsiz}.

We then ran Bonferroni-Holm corrected pairwise comparisons as post-hoc test,
excluding the `First fixation' scenario since the omnibus test was non-significant,
and found that the difference between Q1 vs Q2 was statistically significant in all cases ($p < .001$),
The difference between Q1 vs Q3 and Q1 vs Q4 was statistically significant when users viewed the images for 3 or more seconds ($p < .001$),
The difference between Q2 vs Q3 and Q2 vs Q4 was statistically significant in all cases ($p < .001$).
Finally, the difference between Q3 vs Q4 was significant when users viewed the images for 3 or more seconds ($p=0.018$).

\begin{table}[!ht]
  \centering

  \begin{tabular}{l *4r}
  \toprule
  Viewing time    & $N$ & $\chi^2_{(3, N)}$ & $p$-value & $\phi$ \\
  \midrule
  Up to 1 second  & 109.93 &  90.630 & $<.001$ & 0.908 \\
  Up to 3 seconds & 269.03 & 184.498 & $<.001$ & 0.828 \\
  Up to 7 seconds & 588.84 & 182.134 & $<.001$ & 0.556 \\
  \bottomrule
  \end{tabular}

  \caption{
      Location bias analysis.
      Statistical tests of significance for fixations that occurred in each of the four screen quadrants.
  }
  \label{tbl:quadrants}
\end{table}

\subsubsection{Summary}
We found no center bias, since the distribution of fixations among the quadrants is markedly different.
We found a horizontal bias, since the difference between the number of fixations received in Q1 vs. Q2
are statistically significant in all cases, no matter for how long users were viewing the images,
and between Q3 vs. Q4 when users viewed the images for 3 or more seconds.
Given the observations made, we conclude that there is a strong bias toward the top-left location of the display.

\subsection{Effect of Color}
\label{sec:analysis-color}

We started by checking whether the colors presented and those fixated on follow the same distribution.
The leftmost subplot in \autoref{fig:color_brightness_and_bars} shows the 16 most prevalent colors 
in the original images and the top 16 colors by number of fixations for different time intervals.
Comparison suggests that brighter colors may attract more attention than darker colors.

\begin{figure}[!ht]
\def\w{0.48\linewidth}
\begin{minipage}{\w}
  \includegraphics[width=\textwidth]{results_desktop/color_bias_brightness_boxplot.pdf}
\end{minipage}
\hfill
\begin{minipage}{\w}
 \def\ww{0.48\textwidth}
  \subfloat[All colors]{\includegraphics[width=\ww]{results_desktop/colorhist-img.json_color_bias.png}}\hfill
  \subfloat[Up to 1 second]{\includegraphics[width=\ww]{results/colorhist-fix-first1s.json_color_bias.png}}\hfill
  \subfloat[Up to 3 seconds]{\includegraphics[width=\ww]{results/colorhist-fix-first3s.json_color_bias.png}}\hfill
  \subfloat[Up to 7 seconds]{\includegraphics[width=\ww]{results/colorhist-fix.json_color_bias.png}}
\end{minipage}
\caption{
    Color bias analysis.
    Left: box plots of color brightness for all image colors and for fixated colors at different times.
    Right: displayed colors vs. those fixated upon at different times, sorted by frequency.
}
\label{fig:color_brightness_and_bars}
\end{figure}

To investigate whether a reliable effect exists,
we computed the pixel brightness values by using sRGB Luma coefficients (ITU Rec.\,709)~\cite{bezryadin2007luma},
which reflect the corresponding standard chromaticities,
and compared the distribution of fixation and non-fixation brightness values.
The rightmost subplot in \autoref{fig:color_brightness_and_bars} shows the data.
Bartlett's test of homogeneity of variances showed non-significance in all cases ($T \geq 0.906, p > .05$),
suggesting that brighter colors do not attract significantly more fixations than darker ones.

\subsubsection{Summary}
We did not find a color bias affecting saliency of visual designs.
If attention is drawn to brighter colors, the effect is too modest to be of practical significance.

\section{Location bias per image category}

In the following we break down the analysis provided in \autoref{sec:analysis-location}
by design category, namely: desktop, mobile, web, and poster designs.

\begin{figure*}[!ht]
  \def\w{0.32\linewidth}
  \centering

  \subfloat[Up to 1 second]{\includegraphics[width=\w]{results_desktop/dataset-first1s.csv_location_bias}}\hfill
  \subfloat[Up to 3 seconds]{\includegraphics[width=\w]{results_desktop/dataset-first3s.csv_location_bias}}\hfill
  \subfloat[Up to 7 seconds]{\includegraphics[width=\w]{results_desktop/dataset.csv_location_bias.pdf}}

  \caption{
    Location bias analysis for images in the \textbf{desktop} category.
    The thick dashed lines denote the middle of the screen viewport along the X and Y axis.
  }
  \Description{Color brightness analysis of desktop images.}
  \label{fig:location_bias_desktop}
\end{figure*}

\begin{figure}[!ht]
  \def\w{0.24\linewidth}
  \centering

  \subfloat{\includegraphics[width=\w]{results_desktop/quadrants-first1s.csv_boxplot.pdf}}
  \subfloat{\includegraphics[width=\w]{results_desktop/quadrants-first3s.csv_boxplot.pdf}}
  \subfloat{\includegraphics[width=\w]{results_desktop/quadrants.csv_boxplot.pdf}}

  \caption{
    Location bias analysis for images in the \textbf{desktop} category.
    Distribution of fixations in screen quadrants.
    Q1: top-right, Q2: top-left, Q3: bottom-left, Q4: bottom-right.
  }
  \Description{Quadrant fixations analysis in desktop images.}
  \label{fig:quadrants_desktop}
\end{figure}

\begin{figure*}[!ht]
  \def\w{0.32\linewidth}
  \centering

  \subfloat[Up to 1 second]{\includegraphics[width=\w]{results_mobile/dataset-first1s.csv_location_bias}}\hfill
  \subfloat[Up to 3 seconds]{\includegraphics[width=\w]{results_mobile/dataset-first3s.csv_location_bias}}\hfill
  \subfloat[Up to 7 seconds]{\includegraphics[width=\w]{results_mobile/dataset.csv_location_bias.pdf}}

  \caption{
    Location bias analysis for images in the \textbf{mobile} category.
    The thick dashed lines denote the middle of the screen viewport along the X and Y axis.
  }
  \Description{Color brightness analysis of mobile images.}
  \label{fig:location_bias_mobile}
\end{figure*}

\begin{figure}[!ht]
  \def\w{0.24\linewidth}
  \centering

  \subfloat{\includegraphics[width=\w]{results_mobile/quadrants-first1s.csv_boxplot.pdf}}
  \subfloat{\includegraphics[width=\w]{results_mobile/quadrants-first3s.csv_boxplot.pdf}}
  \subfloat{\includegraphics[width=\w]{results_mobile/quadrants.csv_boxplot.pdf}}

  \caption{
    Location bias analysis for images in the \textbf{mobile} category.
    Distribution of fixations in screen quadrants.
    Q1: top-right, Q2: top-left, Q3: bottom-left, Q4: bottom-right.
  }
  \Description{Quadrant fixations analysis in mobile images.}
  \label{fig:quadrants_mobile}
\end{figure}

\begin{figure*}[!ht]
  \def\w{0.32\linewidth}
  \centering

  \subfloat[Up to 1 second]{\includegraphics[width=\w]{results_web/dataset-first1s.csv_location_bias}}\hfill
  \subfloat[Up to 3 seconds]{\includegraphics[width=\w]{results_web/dataset-first3s.csv_location_bias}}\hfill
  \subfloat[Up to 7 seconds]{\includegraphics[width=\w]{results_web/dataset.csv_location_bias.pdf}}

  \caption{
    Location bias analysis for images in the \textbf{web} category.
    The thick dashed lines denote the middle of the screen viewport along the X and Y axis.
  }
  \Description{Color brightness analysis of web images.}
  \label{fig:location_bias_web}
\end{figure*}

\begin{figure*}[!ht]
  \def\w{0.24\linewidth}
  \centering

  \subfloat{\includegraphics[width=\w]{results_web/quadrants-first1s.csv_boxplot.pdf}}
  \subfloat{\includegraphics[width=\w]{results_web/quadrants-first3s.csv_boxplot.pdf}}
  \subfloat{\includegraphics[width=\w]{results_web/quadrants.csv_boxplot.pdf}}

  \caption{
    Location bias analysis for images in the \textbf{web} category.
    Distribution of fixations in screen quadrants.
    Q1: top-right, Q2: top-left, Q3: bottom-left, Q4: bottom-right.
  }
  \Description{Quadrant fixations analysis in web images.}
  \label{fig:quadrants_web}
\end{figure*}

\begin{figure*}[!ht]
  \def\w{0.32\linewidth}
  \centering

  \subfloat[Up to 1 second]{\includegraphics[width=\w]{results_poster/dataset-first1s.csv_location_bias}}\hfill
  \subfloat[Up to 3 seconds]{\includegraphics[width=\w]{results_poster/dataset-first3s.csv_location_bias}}\hfill
  \subfloat[Up to 7 seconds]{\includegraphics[width=\w]{results_poster/dataset.csv_location_bias.pdf}}

  \caption{
    Location bias analysis for images in the \textbf{poster} category.
    The thick dashed lines denote the middle of the screen viewport along the X and Y axis.
  }
  \Description{Color brightness analysis of poster images.}
  \label{fig:location_bias_poster}
\end{figure*}

\begin{figure}[!ht]
  \def\w{0.24\linewidth}
  \centering

  \subfloat{\includegraphics[width=\w]{results_poster/quadrants-first1s.csv_boxplot.pdf}}
  \subfloat{\includegraphics[width=\w]{results_poster/quadrants-first3s.csv_boxplot.pdf}}
  \subfloat{\includegraphics[width=\w]{results_poster/quadrants.csv_boxplot.pdf}}

  \caption{
    Location bias analysis for images in the \textbf{poster} category.
    Distribution of fixations in screen quadrants.
    Q1: top-right, Q2: top-left, Q3: bottom-left, Q4: bottom-right.
  }
  \Description{Quadrant fixations analysis in poster images.}
  \label{fig:quadrants_poster}
\end{figure}

\clearpage
\section{Color bias per image category}

In the following we break down the analysis provided in \autoref{sec:analysis-color}
by design category, namely: desktop, mobile, web, and poster designs.

\begin{figure}[!ht]
\def\w{0.48\linewidth}
\begin{minipage}{\w}
  \includegraphics[width=\textwidth]{results_desktop/color_bias_brightness_boxplot.pdf}
\end{minipage}
\hfill
\begin{minipage}{\w}
 \def\ww{0.48\textwidth}
  \subfloat[All colors]{\includegraphics[width=\ww]{results_desktop/colorhist-img.json_color_bias.png}}\hfill
  \subfloat[Up to 1 second]{\includegraphics[width=\ww]{results_desktop/colorhist-fix-first1s.json_color_bias.png}}\hfill
  \subfloat[Up to 3 seconds]{\includegraphics[width=\ww]{results_desktop/colorhist-fix-first3s.json_color_bias.png}}\hfill
  \subfloat[Up to 7 seconds]{\includegraphics[width=\ww]{results_desktop/colorhist-fix.json_color_bias.png}}
\end{minipage}
\caption{
    Color bias analysis in \textbf{desktop} images.
    Left: box plots of color brightness for all image colors and for fixated colors at different times.
    Right: displayed (top bar) vs. those fixated upon at different times, sorted by frequency.
}
\label{fig:desktop:color_brightness_and_bars}
\end{figure}

\begin{figure}[!ht]
\def\w{0.48\linewidth}
\begin{minipage}{\w}
  \includegraphics[width=\textwidth]{results_mobile/color_bias_brightness_boxplot.pdf}
\end{minipage}
\hfill
\begin{minipage}{\w}
 \def\ww{0.48\textwidth}
  \subfloat[All colors]{\includegraphics[width=\ww]{results_mobile/colorhist-img.json_color_bias.png}}\hfill
  \subfloat[Up to 1 second]{\includegraphics[width=\ww]{results_mobile/colorhist-fix-first1s.json_color_bias.png}}\hfill
  \subfloat[Up to 3 seconds]{\includegraphics[width=\ww]{results_mobile/colorhist-fix-first3s.json_color_bias.png}}\hfill
  \subfloat[Up to 7 seconds]{\includegraphics[width=\ww]{results_mobile/colorhist-fix.json_color_bias.png}}
\end{minipage}
\caption{
    Color bias analysis in \textbf{mobile} images.
    Left: box plots of color brightness for all image colors and for fixated colors at different times.
    Right: displayed (top bar) vs. those fixated upon at different times, sorted by frequency.
}
\label{fig:mobile:color_brightness_and_bars}
\end{figure}

\begin{figure}[!ht]
\def\w{0.48\linewidth}
\begin{minipage}{\w}
  \includegraphics[width=\textwidth]{results_web/color_bias_brightness_boxplot.pdf}
\end{minipage}
\hfill
\begin{minipage}{\w}
 \def\ww{0.48\textwidth}
  \subfloat[All colors]{\includegraphics[width=\ww]{results_web/colorhist-img.json_color_bias.png}}\hfill
  \subfloat[Up to 1 second]{\includegraphics[width=\ww]{results_web/colorhist-fix-first1s.json_color_bias.png}}\hfill
  \subfloat[Up to 3 seconds]{\includegraphics[width=\ww]{results_web/colorhist-fix-first3s.json_color_bias.png}}\hfill
  \subfloat[Up to 7 seconds]{\includegraphics[width=\ww]{results_web/colorhist-fix.json_color_bias.png}}
\end{minipage}
\caption{
    Color bias analysis in \textbf{web} images.
    Left: box plots of color brightness for all image colors and for fixated colors at different times.
    Right: displayed (top bar) vs. those fixated upon at different times, sorted by frequency.
}
\label{fig:web:color_brightness_and_bars}
\end{figure}

\begin{figure}[!ht]
\def\w{0.48\linewidth}
\begin{minipage}{\w}
  \includegraphics[width=\textwidth]{results_poster/color_bias_brightness_boxplot.pdf}
\end{minipage}
\hfill
\begin{minipage}{\w}
 \def\ww{0.48\textwidth}
  \subfloat[All colors]{\includegraphics[width=\ww]{results_poster/colorhist-img.json_color_bias.png}}\hfill
  \subfloat[Up to 1 second]{\includegraphics[width=\ww]{results_poster/colorhist-fix-first1s.json_color_bias.png}}\hfill
  \subfloat[Up to 3 seconds]{\includegraphics[width=\ww]{results_poster/colorhist-fix-first3s.json_color_bias.png}}\hfill
  \subfloat[Up to 7 seconds]{\includegraphics[width=\ww]{results_poster/colorhist-fix.json_color_bias.png}}
\end{minipage}
\caption{
    Color bias analysis in \textbf{poster} images.
    Left: box plots of color brightness for all image colors and for fixated colors at different times.
    Right: displayed (top bar) vs. those fixated upon at different times, sorted by frequency.
}
\label{fig:poster:color_brightness_and_bars}
\end{figure}
